# Supplementary material for: Rectilinear Link Diameter and Radius in a Rectilinear Polygonal Domain
Source: arXiv:1712.05538 source file (2020-07-03)
Supplement: Supplementary file 1 [file supplement.tex]

\supplement{}%optional, e.g. related research data, source code, ... hosted on a repository like zenodo, figshare, GitHub, ...
